# Supplementary material for: Presentation and Publication: Loss and Slippage in Networks of Automated Market Makers
Source: arXiv:2110.09872 source file (2021-10-18)
Supplement: Supplementary file 1 [file appendix.tex]

Material we may or may not want to include

\section{Appendix}

\subsection{Higher dimensional Capital}

\subsection{Higher dimensional Cost}

\subsection{Divergence Loss and Capitalization}
\daniel{Not sure where this should go,maybe the end of the divergence loss section?}
Suppose that we have an AMM $A$ described by the curve $f$, that is currently in state $(x,f(x))$.
If we want to dynamically modify the AMM curve in between trades it is necessary that $f(x),f'(x)$ remain the same
after a transformation to some $\tilde{f}$.
Here we see that other global quantities must also be preserved.
Define a X-\textit{partition} to be a sequence of elements $\{x_i\}_{i=1}^n$ in $\PosReals$ such that 
\begin{itemize}
    \item $x_1 = x$
    \item $x_i \leq x_j$ $\Leftrightarrow$ $i \leq j$
    \item $\lim_{n \to \infty}x_n = \infty$
\end{itemize}

If we are given a partion $P = \{x_i\}_{i=1}^n$, we then define the total divergence loss wrt to that partition as
\begin{align*}
    L(P,A) = \sum_{i=1}^\infty \divloss^*(x_i,x_{i+1};A)
\end{align*}

Writing this out explicitly gives
\begin{align*}
    &\sum_{i=1}^\infty \divloss^*(x_i,x_{i+1};A) \\
    &= \sum_{i=1}^\infty \bv_{i+1} \cdot (\Phi(\bv_i) - \Phi(\bv_{i+1)}) \\
    &= \sum_{i=1}^\infty \bv_{i+1} \cdot (\Phi(\bv_i) - \Phi(\bv_{i+1)}) \\
    &= \sum_{i=1}^\infty \bv_{i+1} \cdot ((\phi(v_i),f(\phi(v_i))) - (\phi(v_{i+1}),f(\phi(v_{i+1})))) \\
    &= \sum_{i=1}^\infty (v_{i+1},1-v_{i+1}) \cdot (\phi(v_i) - \phi(v_{i+1}),f(\phi(v_i)) - f(\phi(v_{i+1}))) \\
    &= \sum_{i=1}^\infty v_{i+1}(\phi(v_i) - \phi(v_{i+1})) - v_{i+1}(f(\phi(v_i)) - f(\phi(v_{i+1}))) +\sum_{i=1}^\infty f(\phi(v_i)) - f(\phi(v_{i+1})) \\
    &= \sum_{i=1}^\infty v_{i+1}(\phi(v_i) - \phi(v_{i+1})) - v_{i+1}(f(\phi(v_i)) - f(\phi(v_{i+1}))) +f(\phi(v_1)) \\
    &= \sum_{i=1}^\infty v_{i+1}[\phi(v_i) - \phi(v_{i+1}) + f(\phi(v_{i+1})) - f(\phi(v_i))] +f(\phi(v_1)) \\
\end{align*}
Note that each term $\phi(v_i) - \phi(v_{i+1}) + f(\phi(v_{i+1})) - f(\phi(v_i)) \leq 0$.
We also know that $v_1 \geq v_{i+1}$ for each $i$.
This gives us the upper bound
\begin{align*}
    &\sum_{i=1}^\infty v_{i+1}[\phi(v_i) - \phi(v_{i+1}) + f(\phi(v_{i+1})) - f(\phi(v_i))] +f(\phi(v_1)) \\
    &\leq f(\phi(v_1)) = f(x)
\end{align*}
and the lower bound
\begin{align*}
    &\sum_{i=1}^\infty v_{i+1}[\phi(v_i) - \phi(v_{i+1}) + f(\phi(v_{i+1})) - f(\phi(v_i))] +f(\phi(v_1)) \\
    &\geq v_1 \sum_{i=1}^\infty [\phi(v_i) - \phi(v_{i+1}) + f(\phi(v_{i+1})) - f(\phi(v_i))] +f(\phi(v_1)) \\
    &= v_1[\phi(v_1) - f(\phi(v_1))] + f(\phi(v_1)) \\
    &= v_1\phi(v_1) + (1-v_1)f(\phi(v_1)) \\
    &= cap(v;A)
\end{align*}

Simply put
\begin{align*}
    cap(v;A) \leq L(P,A) \leq f(x)
\end{align*}

How tight can this lower bound get?
Well, let $v^{*}$ be the point where $cap(v;A)$ is maximized.
If we let $x^{*} = \phi(v^{*})$, then we know that $f(x^{*}) = x^{*}$.
We know that $cap(v;A) = v^{*}x^{*} + (1-v^{*})f(x^{*}) = f(x^{*})$.
But if $x = x^{*}$ then this means
\begin{align*}
        f(x^{*}) \leq L(P,A) \leq f(x^{*})
\end{align*}
which is entirely independent of the chosen partition $P$, so
\begin{align*}
        f(x^{*}) \leq L(A) \leq f(x^{*})
\end{align*}
or $L(A) = f(x^{*})$.
Additionally, it tells us that total loss is conserved even if we modify the AMM $A$ for $x > x^{*}$.
This makes good intuitive sense, no matter how you choose to drain the reserves by deposing asset type $X$, in the end you will drain all of $f(x^{*})$ if you deposit an infinite amount of $X$.

We can do a similar def for the $y$-axis.
Define a Y-\textit{partition} to be a sequence of elements $\{x_i\}_{i=1}^n$ in $\PosReals$ such that 
\begin{itemize}
    \item $y_1 = f(x)$
    \item $y_i \leq y_j$ $\Leftrightarrow$ $i \leq j$
    \item $\lim_{n \to \infty}y_n = \infty$
\end{itemize}

Let $P_Y = \{y_i\}_{i=1}^{\infty}$ be a Y-partition.
In this case let $g = f^{-1}(x)$.
Here then $y_i = f(x_i)$ so $x_i = f^{-1}(y_i) = g(y_i)$.
Thus $\Phi(\bv_i) = (x_i,f(x_i)) = (g(y_i),f \circ g(y_i) = f \circ f^{-1} (y_i) = y_i$.
That is, $\Phi(\bv_i) = (g(y_i),y_i)$.
The total cost with respect to this partition is
\begin{align*}
    &L(P_Y,A) = \sum_{i=1}^\infty \divloss^*(y_i,y_{i+1};A) \\
\end{align*}
For symmetry in the proof it helps to define $v_i' = 1- v_i$.

This results in
\begin{align*}
    & \sum_{i=1}^\infty \divloss^*(y_i,y_{i+1};A) \\
    &= \sum_{i=1}^\infty \bv_{i+1} \cdot (\Phi(\bv_i) - \Phi(\bv_{i+1)}) \\
    &= \sum_{i=1}^\infty \bv_{i+1} \cdot (g(y_i) - g(y_{i+1}),y_i - y_{i+1})  \\
    &=\sum_{i=1}^\infty (1-v_{i+1}')(g(y_i) - g(y_{i+1}) + v_{i+1}'(y_i - y_{i+1}) \\
    &=\sum_{i=1}^\infty v_{i+1}'[y_i - y_{i+1} +   g(y_{i+1}) - g(y_i)] + \sum_{i=1}^\infty (g(y_i) - g(y_{i+1}) \\
    &=\sum_{i=1}^\infty v_{i+1}'[y_i - y_{i+1} +   g(y_{i+1}) - g(y_i)] + x
\end{align*}
Note that $g(y_i) - g(y_{i+1})) + y_{i+1} - y_i \leq 0$ and $v_1' \geq v_{i+1}'$ for each $i$.
We now get the upper bound
\begin{align*}
    &=\sum_{i=1}^\infty v_{i+1}'[y_i - y_{i+1} +   g(y_{i+1}) - g(y_i)] + x \\
    &\leq x
\end{align*}
and the lower bound
\begin{align*}
    &=\sum_{i=1}^\infty v_{i+1}'[y_i - y_{i+1} +   g(y_{i+1}) - g(y_i)] + x \\
    &\geq v_1'\sum_{i=1}^\infty y_i - y_{i+1} +   g(y_{i+1}) - g(y_i) + x \\
    &= v_1'(y_i - g(y_i)) + x \\
    &= (1-v_i)(f(x_i) - x) + x \\
    &= xv_i (1-v_i)f(x_i) = cap(v;A) 
\end{align*}
So again we get the bounds
\begin{align*}
    cap(v;A) \leq L(P_Y,A) \leq x
\end{align*}

Similar to the $x$-axis case this inequality is tight if $y_1 = f(x^{*})$ and $L(P_Y,A) = x$.
Thus we do get a loss conservation result if we start at $(x^{*},f(x^{*})$.
Namely
\begin{align*}
    L(P_X,A) + L(P_Y,A) = x^{*} + f(x^{*}) = 2x^{*} = 2cap(v^{*};A)
\end{align*}

This has significant meaning to LPs.
The valuation $\bv^{*}$ isn't just a mathematical nicety, it has economic significance.
Namely it is the state for the AMM such that half of the wealth can be lost to $X$ trades and half can be lost to $Y$ trades.

\daniel{TODO: What about when the losses are not centered at the valuation $\bv^{*}$?}
\daniel{TODO: Work out similar result for linear slippage}

\subsection{Optimal AMMs}
If we require that $f(x),f'(x)$ remain the same where $(x,f(x))$ is the current state,
then which AMM optimizes expected capitalization?
For simplicity assume valuations are distributed uniformly.

Thus the expected capitalization is 
\begin{align*}
    &\int_0^1 \bv \cdot \Phi(\bv) dv \\
\end{align*}
Recall that $v = \psi(x)$ so
\begin{align*}
    &\frac{\partial v}{\partial x} = \psi'(x) = \frac{\partial }{\partial x}\frac{f'(x)}{f'(x) - 1} \\
    &= \frac{(f'(x) - 1)f''(x) - f'(x)f''(x)}{(f'(x)) - 1)^2} \\
    &= \frac{-f''(x)}{(f'(x)) - 1)^2}
\end{align*}

So we can do a change of variables to move to the trade space to get
\begin{align*}
    &\int_0^1 \bv \cdot \Phi(\bv) dv \\
    &= \int_0^1 v\phi(v) + (1-v)f(\phi(v)) dv \\
    &= \int_{\infty}^0 [\frac{f'(x)}{f'(x) - 1}x - \frac{1}{f'(x) - 1}f(x)]\frac{-f''(x)}{(f'(x)) - 1)^2} dx \\
    &= \int_{\infty}^0 \frac{f''(x)[f(x) - xf'(x)]}{(f'(x) - 1)^3} dx
\end{align*}

If we think of capitalization as a function of $x,f(x),f'(x),f''(x)$ then maximizing this expected valued is a calculus of variations problem.
Namely, for any AMM $h$ we can write
\begin{align*}
    S[h] = \int_{\infty}^0 F(x,h,h',h'') dx
\end{align*}

where 
\begin{align*}
    & F(x,h,h',h'') = \frac{h''(x)[h(x) - xh'(x)]}{(h'(x) - 1)^3} 
\end{align*}

The Euler-Lagrange equations give a necessary condition for the optimal AMM.
Namely it satisfies this ODE
\begin{align*}
    &\frac{\partial F}{\partial h} - \frac{\partial }{\partial x}(\frac{\partial F}{\partial h'}) + \frac{\partial^2 }{\partial x^2} (\frac{\partial F}{\partial h''}) = 0
\end{align*}
that is
\begin{align*}
    h''(x)(2 + h'(x) - 3xh''(x)) + (h'(x) - 1)xh'''(x) = 0
\end{align*}

subject to the 3 boundary conditions
\begin{itemize}
    \item $h(x) = f(x)$
    \item $h'(x) = f'(x)$
    \item $h''(x) = f''(x)$
\end{itemize}

\subsection{Long Derivations}
express $\linslip$ in terms of $v_1,v_2,v_3$
\begin{align*}
  \linslip_X(v_{12},v_{12}'; A)
  &= \left(\frac{1-v_{12}'}{1-v_{12}}\right)\left( \bv_{12} \cdot \Phi(v_{12}')
  - \bv_{12} \cdot \Phi(v_{12}) \right) \\
  &= \left(\frac{1-\frac{v_1'}{v_1'+v_2'}}{1-\frac{v_1}{v_1+v_2}}\right)\left( \bv_{12} \cdot \Phi(v_{12}')
  - \bv_{12} \cdot \Phi(v_{12}) \right) \\
  &= \left(\frac{\frac{v_2'}{v_1'+v_2'}}{\frac{v_2}{v_1+v_2}}\right)\left( \bv_{12} \cdot \Phi(v_{12}')
  - \bv_{12} \cdot \Phi(v_{12}) \right) \\
  &= \left(\frac{v_2'}{v_2}\right)
  \left( \frac{v_1+v_2}{v_1'+v_2'}\right)
  \left( \bv_{12} \cdot \Phi(v_{12}') - \bv_{12} \cdot \Phi(v_{12}) \right) 
\end{align*}
long derivation of \eqnref{linslipyz}
\begin{alignat}{1}
&v_3' \left(
(f(x)-(x+\delta))g'(y)
+ g(y+f(x)-(x+\delta))
- g(y)
\right)\\
&=
v_3' \left(
(f(x)-(x+\delta))\frac{v_2}{v_3}
+ g(y+f(x)-(x+\delta))
- g(y)
\right)\\
&=
\frac{v_3'}{v_3}
\left(
v_3(f(x)-(x+\delta))
+ v_2(g(y+f(x)-(x+\delta))
- g(y))
\right)\\
&=
\frac{v_3'}{v_3}
\left(
v_3(\phi_2(v_{23})-(x+\delta))
+ v_2(g(y+f(x)-(x+\delta))
- g(y))
\right)\\
&=
\frac{v_3'}{v_3}
\left(
v_3(\phi_2(v_{23})-\phi_2(v_{23}'))
+ v_2(g(y+f(x)-(x+\delta))
- g(y))
\right)\\
&=
\frac{v_3'}{v_3}
\left(
v_3(\phi_2(v_{23})-\phi_2(v_{23}'))
+ v_2(g(\phi_2(v_{23}'))
- g(y))
\right)\\
&=
\frac{v_3'}{v_3}
\left(
v_3(\phi_2(v_{23})-\phi_2(v_{23}'))
+ v_2(g(\phi_2(v_{23}'))
- g(\phi_2(v_{23}))
\right)\\
&=
\frac{v_3'}{v_3}
(v_2+v_3)
\left(
\frac{v_3}{v_2+v_3}(\phi_2(v_{23})-\phi_2(v_{23}'))
+ \frac{v_2}{v_2+v_3}(g(\phi_2(v_{23}'))
- g(\phi_2(v_{23}))
\right)\\
&=
\frac{v_3'}{v_3}
(v_2+v_3)
\left(
\bv_{23} \cdot \Phi_2(\bv_{23}')- \bv_{23} \cdot \Phi_2(\bv_{23}))
\right)\\
&=
(v_2'+v_3') \linslip_X(v_{23},v_{23}').
\end{alignat}
